# Supplementary material for: VGX: Large-Scale Sample Generation for Boosting Learning-Based Software Vulnerability Analyses
Source: arXiv:2310.15436 source file (2024-01-04)
Supplement: Supplementary file 1 [file appendix.tex]

\section{Pattern Refinement}\label{sec:manualpatterns}
%To do the refinement, we apply the 300 filtered patterns to the vulnerability-introducing training samples. This results in false positives (the pattern is applied but the generated sample is not vulnerable) and false negatives (none of the 300 patterns can be applied) against some samples. 
For pattern refinement, we applied the 300 filtered patterns to the vulnerability-introducing training samples. As a result, we encountered \textit{false positives}, where the pattern was applied but the generated sample was not actually vulnerable, as well as \textit{false negatives}, where none of the 300 patterns could be applied.

For the false positives, we consider that the patterns applied on them are \ul{too general}. 
We then removed the patterns against which more than half of the applications are false positives. %and they are the 21 patterns actually removed. 
%We removed patterns that resulted in more than half of the false positive applications. 
In total, we removed 21 patterns in this manner.

For the false negatives, we consider that the %existing 
corrresponding 
patterns are \ul{too specific}. Thus, we need to \ul{manually define new patterns} that are necessarily more general. 
%To do so, we check the commit message associated with the false negative and find the respective CWE ID~\cite{cwereport} for that sample. 
To do so, we examined the commit messages associated with false negatives and identified the corresponding CWE IDs for the corresponding sample using the CWE report~\cite{cwereport}
Then, we read the CWE document and check the synthetic examples used to describe the CWE ID. We also go to the CVE/NVD database~\cite{nvd} to check other real-world vulnerability samples with the same CWE ID. Based on the false negative, the synthetic example, and other real-world samples, we %imagine 
compose/envision 
several possible patterns that can cover them. %in our brains. 
Then, we go back to the existing pattern set and find patterns close to the %imagined 
envisioned 
ones. We finally modify these patterns into the envisoned patterns with the use of regular expression (regex). These modified patterns are the 20 manually defined new patterns described in Table~\ref{tab:derived-patterns}. For example, we notice that there are many false negatives happening on project-defined functions for freeing/releasing pointers (e.g., Figure~\ref{fig:case-re}). It is difficult for the patterns to cover all these statements. Thus, we manually define patterns with regular expressions so that once the function-call name involves pointer freeing keywords like "free", "release", etc., we can match and apply the patterns.

% To define these patterns, we carefully check the 300 filtered patterns, the real-world vulnerability fixes in the training set, and the top-25 most dangerous vulnerability types in the CWE catalog~\cite{cwereport}. We analyze whether those 300 %filtered 
% patterns indeed cover all the common types of real-world vulnerability injection edits. 
% If not, we inspected the training samples and the examples shown in the CWE catalog to derive patterns that can apply on them. Based on our observations, we find that regular expression (regex) is necessary in the patterns. For example, there are many project-defined functions for freeing/releasing pointers. It is difficult for the patterns to cover all these statements. Thus, we derive patterns with regular expressions so that once the function-call name involves "free", "release", etc., we can match and apply them. Table~\ref{tab:derived-patterns} shows the 20 patterns we derive and the respective justifications for them. 
\begin{table}[htbp]
  \centering
  \caption{Manually Defined Patterns}
    \scalebox{0.9}{
        \begin{tabular}{|p{14em}|p{15em}|}
        \hline
        Manually derived pattern & Justification \\
        \hline
        *mutex*(h0); => EMPTY & 
        “Race Condition” mostly happens with a lack of mutex related statements, but there are many  mutex related function~\cite{race-condition}. Thus, once the located statement involve “mutex”, we delete it. \\
        \hline
        *TCHECK*(h0); => EMPTY & There are many samples in the train- \\
        *assert*(h0); => EMPTY & ing set deleting statements involving "TCHECK" and "assert", but they usually use different function names\cite{tcheck}. Thus, once located statement involve “TCHECK” or “assert”, we delete it. \\ 
        \hline
        *free*(h0); => EMPTY & "Memory Leak" mostly happens with   \\
        *Free*(h0); => EMPTY & not releasing assigned memory. \\
        *destruct*(h0); => EMPTY &  However, there may be many differ-  \\
        *destroy*(h0); => EMPTY & ent functions for releasing the mem-  \\
        *unref*(h0); => EMPTY & ory~\cite{memleak}. Thus, once the the located   \\
        *clear*(h0); => EMPTY & statement involve memory release related functions, we delete it. \\
        \hline
        static h0 h1 = h2; => h0 h1 = h2; & "Type Error" usually happens with  \\
        unsigned h0; => h0; & not using static, unsigned, large-size  \\
        int64\_t h0; => int h0; & types, but the current patterns specify too many details like identifier names or assigned values in the patterns~\cite{typeerr}. Thus, we make these details holes so that they are more general.  \\
        \hline
        memset(h0); => EMPTY & "Use of Uninitialized Variables" usu-\\
        h0 = *ERR*; => EMPTY & ally happens with not initializing de- \\
        h0 = *NONE* => EMPTY & clared variables, but current  \\
        h0 = 0; => EMPTY & patterns specify too many details like \\
        h0 = NULL; => EMPTY &  identifier names and values in the \\
        *buf* = h0; => EMPTY &  patterns~\cite{uninit}. Thus, we make these details holes and use regular expression to represent the common initialized value, so that they are more general. \\
         \hline
        h0 = kcalloc(hole1, hole2, hole3);  & "Memory Allocation Vulnerability"  \\
                    \hspace{0.5em} => h0 = kzalloc(h1*h2, h3); & usually happens when using unsafe memory allocation functions, but \\
        h0 = calloc(hole0, hole1);  &  current patterns specify too many de- \\
                   \hspace{0.5em} => h0 = malloc(h1*h2); & tails like identifier names and values in the patterns~\cite{allocerr}. Thus, we make them holes to make the patterns more general. \\
        \hline
        \end{tabular}
    }
    \label{tab:derived-patterns}
\end{table}

\begin{table*}[htbp]
  \centering
  \caption{Pattern Mutation Rules}
    \scalebox{0.96}{
    \begin{tabular}{|p{40em}|p{20em}|}
    \hline
    Pattern Mutation Rule & Justification \\
    \hline
    \textbf{Function call return value assignment mutation:} & Some function calls like strncpy may return some  \\
    function\_call\_name(parameters); => new\_function\_call\_name(new\_parameters); & values but the return values do not always assign  \\
    \hspace{5em}$\Updownarrow$ & to a variable. Mutating such patterns so that they  \\
     h0=function\_call\_name(parameters); => h0=new\_function\_call\_name(new\_parameters);& have or remove the return value assignments increases the generalizability of the pattern set.\\
    \hline
    \textbf{Returned error code mutation:} & The typical safety issue checks do some check  \\
    if(condition) {return NULL;} => EMPTY & in an if statement condition and then return  \\
    \hspace{5em}$\Updownarrow$ & an error code when found the issue. However,  \\
    if(condition) {return 0;} => EMPTY & there are many possible returned error codes. We  \\
    \hspace{5em}$\Updownarrow$& mutate these returned error codes to make the  \\
    if(condition) {return;} => EMPTY & patterns more general. \\
    \hspace{5em}$\Updownarrow$&  \\
    if(condition) {return -1;} => EMPTY &  \\
    \hspace{5em}$\Updownarrow$&  \\
    if(condition) {return -EINVAL/EBADFD/ENOTSOCK/EPERM/ENODEV/ENOMEM;} =>  EMPTY &  \\
    \hline
    \textbf{Safety check condition generalization mutation:} & In our automatic pattern mining, the mined safety  \\
    if(specific\_condition) {return error\_code;} => EMPTY & checks if statements may be too specific in the \\
    \hspace{5em}$\Downarrow$& condition. However, if an if statement only has  \\
    if(hole) {return error\_code;} => EMPTY & one return statement, it is very likely that it is a safety check if statement. Thus, we remove the specific conditions in these if statements and use a hole to make the patterns more general. \\
    \hline
    \textbf{Safety check exit statement mutation:} & When the safety checks if statements find issues,  \\
    if(condition) {return error\_code;} => EMPTY & they may not always exit the function using  \\
    \hspace{5em}$\Updownarrow$& a return statement. If the safety check is in a \\
    if(condition) {break;} => EMPTY & for/while/switch block, it may use a break or  \\
    \hspace{5em}$\Updownarrow$& continue statement to exit. Thus, we mutate the  \\
    if(condition) {continue;} => EMPTY & exit statement to make the patterns more general. \\
    \hline
    \end{tabular}}
  \label{tab:mutation}
\end{table*}

\section{Manually Deriving Pattern Mutation Rules}\label{sec:manualmutationrules}
%To derive the rules, we carefully check the refined pattern set with 299 edit patterns, as well as the real-world vulnerability fixes in the training set and the top-25 most dangerous vulnerability types in CWE~\cite{cwereport}. 

To derive the \ul{pattern mutation rules} that make the existing patterns more general but not too general, we carefully check the traditional mutation operators for C language~\cite{agrawal1989design}. We select those without changing the code functionality significantly and finally derive four types of pattern mutation rules: \textit{function call return value assignment mutation}, \textit{returned error code mutation}, \textit{safety check condition generalization mutation}, and \textit{safety check exist statement mutation}. Table~\ref{tab:mutation} shows the pattern mutation rules we derived and the respective justifications for them. $\Updownarrow$ means the mutation is bidirectional, while $\Downarrow$ means the mutation is unidirectional.

%We observe and analyze whether the edit patterns are safe to add, modify, or deleting some code elements without making them too general. Based on our observation, we notice that it is safe to add or delete the return value assignment, change the returned error code, make the specific condition in a safety check condition a general placeholder (hole), and change the exit statement in a safety checking if-statement. Table~\ref{tab:mutation} shows the pattern mutation rules we derive and the respective justifications for them. $\Updownarrow$ means the mutation is bidirectional, while $\Downarrow$ means the mutation is unidirectional.

\section{Latest CVEs Detected by the Models}\label{sec:cves}
We scrape the latest 71 vulnerabilities (CVEs) covering 17 CWEs from 6 critical software projects (e.g., Linux kernel) reported between 2021-2023, from the CVE/NVD database~\cite{nvd}. Table~\ref{tab:cve} shows these latest vulnerabilities detected by LineVul before and after the improvement. The rows marked green are those detected by the improved model but cannot be detected by the original model. The improved LineVul found 13 more vulnerabilities (CVEs), indicating the potential ability of the improved model to detect real-world, zero-day vulnerabilities.

\begin{table}[htbp]
  \centering
  \caption{Latest CVEs Detected}
    \scalebox{0.95}{
    \begin{tabular}{|l|c|c|}
    
    \hline
    \textbf{CVE}   & \textbf{LineVul-ori} & \textbf{LineVul-aug} \\ \hline
   \rowcolor{green!30} 2022-46149 &X    &$\checkmark$\\ \hline
   \rowcolor{green!30} 2023-27478 &X    &$\checkmark$\\ \hline
    2022-39188 &X    &X\\ \hline
    2022-47518 &$\checkmark$    &$\checkmark$\\ \hline
    2023-23001 &$\checkmark$    &$\checkmark$\\ \hline
   \rowcolor{green!30} 2022-28388 &X    &$\checkmark$\\ \hline
    2023-23005 &$\checkmark$    &$\checkmark$\\ \hline
   \rowcolor{green!30} 2023-22996 &X    &$\checkmark$\\ \hline
    2022-1199 &$\checkmark$    &$\checkmark$\\ \hline
    2023-23006 &$\checkmark$    &$\checkmark$\\ \hline
   \rowcolor{green!30} 2021-3743 &X    &$\checkmark$\\ \hline
    2022-1199 &$\checkmark$    &$\checkmark$\\ \hline
    2022-47942 &$\checkmark$    &$\checkmark$\\ \hline
    2022-1353 &$\checkmark$    &$\checkmark$\\ \hline
    2022-40307 &X    &X\\ \hline
    2023-1118 &$\checkmark$    &$\checkmark$\\ \hline
    2022-24959 &$\checkmark$    &$\checkmark$\\ \hline
    2022-25375 &$\checkmark$    &$\checkmark$\\ \hline
    2023-22997 &$\checkmark$    &$\checkmark$\\ \hline
    2023-23000 &$\checkmark$    &$\checkmark$\\ \hline
    2022-47519 &$\checkmark$    &$\checkmark$\\ \hline
    2022-24958 &$\checkmark$    &$\checkmark$\\ \hline
    2022-36123 &$\checkmark$    &$\checkmark$\\ \hline
    2021-3640 &$\checkmark$    &$\checkmark$\\ \hline
    2022-47940 &$\checkmark$    &$\checkmark$\\ \hline
    2022-2959 &$\checkmark$    &$\checkmark$\\ \hline
   \rowcolor{green!30} 2022-24958 &X    &$\checkmark$\\ \hline
   \rowcolor{green!30} 2021-3764 &X    &$\checkmark$\\ \hline
    2022-3424 &$\checkmark$    &$\checkmark$\\ \hline
    2023-0030 &X    &X\\ \hline
   \rowcolor{green!30} 2022-47938 &X    &$\checkmark$\\ \hline
    2022-1975 &$\checkmark$    &$\checkmark$\\ \hline
    2020-36691 &$\checkmark$    &$\checkmark$\\ \hline
    2022-29156 &$\checkmark$    &$\checkmark$\\ \hline
    2022-29156 &$\checkmark$    &$\checkmark$\\ \hline
    2023-23004 &$\checkmark$    &$\checkmark$\\ \hline
    2022-33981 &$\checkmark$    &$\checkmark$\\ \hline
    2022-34494 &$\checkmark$    &$\checkmark$\\ \hline
    2022-42703 &$\checkmark$    &$\checkmark$\\ \hline
   \rowcolor{green!30} 2023-23002 &X    &$\checkmark$\\ \hline
    2022-39842 &$\checkmark$    &$\checkmark$\\ \hline
    2022-1043 &$\checkmark$    &$\checkmark$\\ \hline
    2022-3202 &$\checkmark$    &$\checkmark$\\ \hline
    2022-47943 &X    &X\\ \hline
   \rowcolor{green!30} 2022-42895 &X    &$\checkmark$\\ \hline
    2022-2153 &$\checkmark$    &$\checkmark$\\ \hline
    2023-22999 &X    &X\\ \hline
    2023-1390 &$\checkmark$    &$\checkmark$\\ \hline
   \rowcolor{green!30} 2022-34495 &X    &$\checkmark$\\ \hline
    2023-22998 &$\checkmark$    &$\checkmark$\\ \hline
    2022-28390 &X    &X\\ \hline
    2022-28796 &$\checkmark$    &$\checkmark$\\ \hline
   \rowcolor{green!30} 2022-47520 &X    &$\checkmark$\\ \hline
    2023-28772 &$\checkmark$    &$\checkmark$\\ \hline
    2021-3609 &$\checkmark$    &$\checkmark$\\ \hline
    2022-1974 &$\checkmark$    &$\checkmark$\\ \hline
    2021-3736 &$\checkmark$    &$\checkmark$\\ \hline
    2022-29582 &$\checkmark$    &$\checkmark$\\ \hline
    2022-41858 &$\checkmark$    &$\checkmark$\\ \hline
   \rowcolor{green!30} 2022-30594 &X    &$\checkmark$\\ \hline
    2022-47521 &$\checkmark$    &$\checkmark$\\ \hline
    2022-36879 &$\checkmark$    &$\checkmark$\\ \hline
    2023-22995 &$\checkmark$    &$\checkmark$\\ \hline
    2022-1205 &$\checkmark$    &$\checkmark$\\ \hline
    2022-1852 &$\checkmark$    &$\checkmark$\\ \hline
    \textbf{Total} & \textbf{49}    & \textbf{62} \\ \hline 
    \end{tabular}}
  \label{tab:cve}
\end{table}%

\section{Statistics/Metadata of the Generated Dataset}\label{sec:datastatistics}
As part of the contributions of this paper, we provide and will (responsibly) share our dataset of 150,392 vulnerable samples. 
In this dataset, each vulnerable sample is accompanied by the following kinds of related information that is valuable for various downstream vulnerability analysis tasks:
\begin{itemize}
    \item \textbf{Paired normal sample}: for each vulnerable sample, the corresponding normal (i.e., vulnerability-fixed) sample is included. The availability of the pairings is useful for developing both vulnerability detection and vulnerability repair techniques especially those that are data-driven (i.e., DL-based). 
    \item \textbf{Vulnerability location}: per the nature of our {\tech} design, the location information of each generated vulnerable sample is naturally available. This fine-grained information (i.e., which particular code lines are vulnerable) is essential for developing vulnerability localization techniques based on such samples. 
    \item \textbf{Vulnerability type}: for each generated vulnerable sample, {\tech} automatically assigns the sample's vulnerability type label as that assigned for the injection edit pattern that was used for generating the sample. The availability of this label is essential for using our samples to develop fine-grained vulnerability analysis such as vulnerability classification. 
    \item \textbf{Associated software project}: for each generated sample, {\tech} automatically associates it with the software project to which the corresponding normal sample belongs. This information is useful for optimizing some downstream vulnerability analysis (e.g., within-project vulnerability prediction and vulnerability-based project clustering).
\end{itemize}

Currently, the 150,392 vulnerable samples in our dataset already represent 238 different software projects. Apparently, the diversity of our dataset in this regard depends on that of the 
input normal samples. 
Similarly, the diversity of our datasets in terms of vulnerability type (e.g., CWE) coverage depends on that of the injection edit patterns.

\section{Ethical Disclosures}
The goal of this work is to help address the urgent needs for large-scale high-quality vulnerability datasets for the purpose of developing more powerful/effective defensie techniques, not at all meant to benefit adversarial ends. 
The vulnerable samples we generated would not cause ethical issues for severa reasons. 
First, these samples will not be deployed in any way and the vulnerabilities are not in real-world software that has been or will be deployed. 
%Second, the samples will not be disclosed to users
Second, no exploits for any of the generated vulnerabilities are provided. 
Third, in the unlikely cases in which attackers get access to the samples hence utilizing 
the vulnerabilities in them against real-world software, 
such vulnerabilities would be highly detectable by 
models trained on those samples.
